# Supplementary material for: Three addressable spin qubits in a molecular single-ion magnet
Source: arXiv:1610.03994 source file (2016-10-13)
Supplement: Supplementary file 1 [file Jenkins_v1_supplementary.pdf]

# Supplementary information

# Three addressable spin qubits in a molecular single-ion magnet

M. D. Jenkins, Y. Duan, B. Diosdado, J. J. García-Ripoll, A. Gaita-Ariño, C. Giménez-Saiz, P. J. Alonso, E. Coronado, F. Luis

## Experimental details

**Synthesis** Samples of $K_{12}[Gd(H_2O)P_5W_{30}O_{110}]\cdot 27.5H_2O$ ($GdW_{30}$) and $K_{12}[Y(H_2O)P_5W_{30}O_{110}]\cdot 29H_2O$ ($YW_{30}$) were prepared by adaptations of previously reported methods.[S1] Samples of magnetically diluted systems (potassium salts of $[Gd_xY_{1-x}(H_2O)P_5W_{30}O_{110}]^{12-}$, referred to as $Y_{1-x}Gd_xW_{30}$ with $x$ = 0.01 and 0.05), were prepared by dissolving pure crystal samples of $GdW_{30}$ and $YW_{30}$ in the proper molar ratio at 80°C. Crystals of $Y_{1-x}Gd_xW_{30}$ were obtained from these solutions after several days standing in open beakers at room temperature. The chemical compositions were evaluated by Inductively Coupled Plasma-atomic emission spectroscopy.

**X-ray diffraction** Suitable crystals of $GdW_{30}$, $YW_{30}$, and $Gd_xY_{1-x}W_{30}$ ($x$ = 0.01 and 0.05) were taken from solution, coated with Paratone N oil, suspended on small fiber loops, and placed in a stream of cooled nitrogen (120 K) on an Oxford Diffraction diffractometer equipped with a graphite-monochromated enhanced (Mo) X-ray Source ($\lambda$ = 0.71073 Å). For $GdW_{30}$ and $YW_{30}$, data collection routines, unit cell refinements, and data processing were carried out using the CrysAlis software package developed by Agilent Technologies. The structure solution and refinement were carried out using SHELXS-97 and SHELXL-

2014.[S2] The crystal structure is shown in Fig. S1 and the crystallographic data are listed in Table S1. For $Gd_xY_{1-x}W_{30}$ ($x$ = 0.01 and 0.05) X-ray powder diffractograms indicate that all compounds have the same cell parameters (Table S2) and are therefore isostructural. X-ray diffraction experiments were also performed on single crystals of $Y_{0.99}Gd_{0.01}W_{30}$. Results are shown in Fig. S2. They are compatible with the orthorhombic crystal structure of the undiluted $GdW_{30}$, with lattice parameters $a$ = 28.814 Å, $b$ = 21.411 Å, and $c$ = 20.825 Å.

**EPR experiments** Continuous wave (cw) and pulsed time domain (TD) Electron Paramagnetic Resonance (EPR) measurements were performed with a Bruker Biospin ELEXSYS E-580 spectrometer operating in X-band (9-10 GHz). The temperature of the sample was varied between 6 K and 300 K using gas-flow Helium cryostats. Polycrystalline samples were introduced in quartz tubes and sealed under an Ar atmosphere. Some cw EPR spectra measured on these samples are shown in Fig. S3. Fits of these curves allow the determination of the $D$ and $E$ magnetic anisotropy parameters. The inhomogeneous broadening seems to be dominated, at low temperatures, by sizeable distributions of these parameters, which are probably associated with the freezing of vibrational modes or with some disorder in the locations of water molecules. Single crystals (typically 1×0.3×0.3 mm) were glued on a 2×2×2 mm nylon cube with their **a** crystallographic axis parallel to one of the cube's edges. The cube was mounted on a sample holder that can be rotated around the vertical laboratory axis in order to measure the angular dependence of the cw-EPR spectra (Fig. S4) and to get the desired orientation of the crystal with respect to the magnetic field for the TD experiments. On-chip EPR experiments were performed by coupling single crystals of undiluted $GdW_{30}$ to superconducting coplanar waveguides and 1.5 GHz resonators. These devices are fabricated

on 500 μm thick C-plane sapphire wafers and consist of a 150 nm thick niobium layer deposited by radio frequency (RF) sputtering and then patterned by either photolithography and lift-off or reactive ion etching. The external magnetic field was oriented in situ with a 9T×1T×1T superconducting vector magnet. Some representative results are shown in Figs. S5 and S6. Finally, the relaxation of the electronic spin echo (ESE )measured in two-pulse and three-pulse TD experiments, which give $T_2$ and $T_1$ relaxation times, are shown in Figs. S7a and S7b.

**Spin nutation experiments** The spin nutation signals of different $Y_{0.99}Gd_{0.01}W_{30}$ single crystals have been obtained by measuring the amplitude of the ESE generated by the application of a two-pulse sequence: $p(t_p)$ - $\tau$ - $p(\pi)$ - $\tau$ - ESE as a function of the first pulse length $t_p$.[S3] In a particular experiment, the interval τ between the two pulses was kept fixed (typically 120 to 200 ns) and the length of the π pulse was adjusted to maximize the echo amplitude for each high power attenuation value (HPA). This pulse is also sufficiently short (less than 40 ns) to ensure that the hard pulse approximation describes well the spin dynamics taking place under its influence. The measured signal is then proportional to the *y* spin component (in the rotating system), $S_y(t_p)$, generated by the nutation pulse $p(t_p)$.

By contrast, the length of the nutation pulse can significantly exceed $T_2$. The ensuing spin dynamics and the actual pulse shapes must therefore be explicitly taken into account. The ideal description as a square-shaped pulse becomes a good approximation for sufficiently long pulses. However, for low $t_p$ values (typically less than 100 ns) the actual shape departs significantly from this description. For this reason, besides other considerations on the spectral excitation that are discussed below, the analysis of the nutation signal takes into account data measured for $t_p$ larger than an onset $t_{p0}$; typically $t_{p0}$ = 100 ns. It has also been

checked that the relative height of the "flat region" of the "in phase" excitation pulse follows the expected exponential dependence on HPA.

## Analysis of spin nutation signals

**Modelling of the nutation signal.** As can be seen in the Zeeman energy diagram shown in Fig. 1 of the main text, the two levels involved in any EPR transition are well isolated from the rest. The Bloch formalism can then be safely used for a phenomenological description of the experiments. These experiments measure the time evolution of $S_y(t_p)$, the component of the magnetization in the rotating frame that is perpendicular to the static magnetic field and to the microwave magnetic field. The initial values of $\boldsymbol{S}$ are assumed to be given by $S_x(0) = S_y(0) = 0$ and $S_z(0) = S_0$, the equilibrium spin polarization in a static magnetic field $H_z$. In what follows, it is also assumed that $\Omega_{R,n} \equiv g\mu_B|\langle n|2S_x|n+1\rangle|h_1 >> \delta_n, T_2^{-1}, T_1^{-1}$, where $\delta_n \equiv \Delta_n/\hbar\text{-}\omega$ is the detuning of the n-th transition from the microwave driving frequency ω. The first of these conditions holds provided that $t_p >> 2\pi/\Omega_{R,n}^{-1}$, because such long pulses excite only spins in or very near resonance. On the other hand, $1/T_2$ is about 2 MHz and $1/T_1$ about 0.4 MHz (see Fig 2b) for all transitions while the nutation frequencies range from 10 to 30 MHz depending of the power. Under these conditions, $S_y(t_p)$ can be expressed as follows[S3]

$$S_y(t_p;\delta_n) \cong S_0 e^{-t_p/T_2} \frac{\Omega_{R,n}}{\sqrt{\Omega_{R,n}^2+\delta_n^2}} exp\left[\frac{1}{2}\left(\frac{1}{T_2}-\frac{1}{T_1}\right)\frac{\Omega_{R,n}^2}{\Omega_{R,n}^2+\delta_n^2}t_p\right] \times \\ sin\left(\sqrt{\Omega_{R,n}^2+\delta_n^2}\,t_p\right) + S_y^{no}(t_p;\delta_n) \qquad \text{(S1)}$$

where $S_y^{no}(t,\delta_n) = ae^{-\gamma t_p} + S_y^{st}$ is a non oscillatory contribution,

$a = \frac{\left(T_2^{-1} - T_1^{-1}\right)^3 \Omega_{R,n}^3 \delta_n}{\left(\Omega_{R,n}^2 + \delta_n^2\right)^2 \left(T_2^{-1}\Omega_{R,n}^2 + T_1^{-1}\delta_n^2\right)} S_0$, $\gamma \approx \frac{1}{T_2} - \left(\frac{1}{T_2} - \frac{1}{T_1}\right)\frac{\delta_n^2}{\Omega_{R,n}^2 + \delta_n^2}$ and $S_y^{st}$ is the stationary state solution (the cw EPR signal). In a real sample, each resonance line has some inhomogeneous broadening characterized by a normalized line shape function $g(\delta_n)$ that fulfills $\int g(\delta_n)d\delta_n = 1$ and $\int \delta_n g(\delta_n)d\delta_n = 0$. A measure of this broadening is given by $\sigma$, with $\sigma^2 = \int \delta_n^2 g(\delta_n)d\delta_n$. The nutation signal $S_y(t_p)$ is then obtained as the average $S_y(t_p) = \int S_y(t_p;\delta_n) g(\delta_n) d\delta_n$ of $S_y(t_p;\delta_n)$ weighted by the distribution $g(\delta_n)$. When, as it is the case with $GdW_{30}$, $\sigma >> \Omega_{R,n}$, $S_y(t_p)$ can be described as:[S4-S6]

$$S_y(t_p) = K_n e^{-t_p/\tau_{R,n}} J_0(\Omega_{R,n} t_p) + S_y^{no} \qquad \text{(S2)}$$

where $K_n$ is a constant, $J_0$ is the Bessel function of first kind and the damping time $\tau_{R,n}$ depends on the microwave power as $\frac{1}{\tau_{R,n}} = \alpha + \beta\Omega_{R,n}$ with $\alpha$ and $\beta$ constant parameters and $\alpha \geq 1/2T_2$. This dependence was first observed experimentally by Boscarino and co-workers[S7,S8] for E' centers in glassy silica and for $[AlO_4]^0$ centres in quartz. The observation of this non-Bloch behavior for high values of the driving field (high values of the Rabi frequency) led to the development of some phenomenological models.[S9,S10] In particular, Shakmuratov and co-workers[S9] described this behavior by introducing fluctuations in the amplitude and phases of the driving magnetic field, and tentatively associated such fluctuations with dipolar interactions between electronic spins. Their model leads to a damping of the Rabi oscillation as that given by Eq. (S2) with $\alpha = (1/T_1 + 1/T_2)/2$. For $T_2 << T_1$ this expression simplifies to $\alpha = 1/2T_2$, which is often used in the

literature. Further studies of E' centers in silica[S11] showed that the $\beta$ parameter depends on the concentration of paramagnetic entities, thus supporting the hypothesis that the stochastic field responsible for the "anomalous decay" of the nutation signal is due to dipolar interactions. Such a concentration dependence of $\beta$ (and $\tau_{R,n}$) has been observed in several diluted paramagnetic systems.[S12] In addition to dipolar interactions, some other contributions arising from, e.g., inhomogeneities in the microwave magnetic field $h_1$ throughout the sample have to be considered.[S12] Baibekov and co-workers worked out a detailed theoretical model that takes into account dipole-dipole, electrostatic, and hyperfine interactions.[S5,S12,S13] The influence of these effects on the decay of Rabi oscillations has also been confirmed by numerical simulations.[S14] It follows from these studies that, in a limited region of $\Omega_{R,n}$, the dependence of $1/\tau_{R,n}$ on the Rabi frequency is linear and that $\alpha \approx (1/T_1 + 1/T_2)/2$.

The Bessel function $J_0$ leads also to a faster decay of spin oscillations as compared with a pure sinusoidal function. This additional decay reflects the fact that, in a sample with a sizeable inhomogeneous broadening described by $g(\delta_n)$, the fraction of all spins that gets excited by the nutation pulse decreases as the pulse length increases.

For a single crystal of $Y_{0.99}Gd_{0.01}W_{30}$, the peak to peak widths of the cw-EPR lines (see Fig. 1a) lie in between 10 and 20 mT (depending on the transition). Using a Gaussian line shape, this results in $\sigma > 150$ MHz. Consequently, the above approximation can be safely used to describe spin nutation signals measured in this material, taking into account that, in all cases, nutation frequencies remain lower than 30 MHz.

The non-oscillatory contribution consists of two parts: one of them is constant and corresponds to the steady-state value $S_y^{st}$, while the other decays with time. Let us focus on

the latter contribution $S_y$', which vanishes in the case of an ideal experiment and for exact resonance ($\delta_n = 0$). If the inhomogeneous broadening is symmetric and the magnetic field is tuned to the center of the resonance line, $g(\delta_n)$ is an even function and, consequently, $S'_y(t_p)$ will also be zero, since $\gamma$ is an even function of $\delta_n$ whereas $a$ is an odd function. In practice, it is not possible to set the magnetic field value with arbitrary accuracy. Besides, the line shape can be asymmetric, as it is the case when the inhomogeneous broadening results from distributions of the magnetic anisotropy parameters (or the zero-field splittings). This effect is likely present in $GdW_{30}$ molecules at low temperatures (see Fig. S3) and accounts for the increase of the resonance line widths as one moves from the center of the spectrum to its wings. In addition, the excitation with non-ideal pulses, which have a significant "out of phase" contribution, mainly in its ends, can introduce some mixing of $S_y$ with other magnetization components in the rotating frame.

The damping constant $\gamma$ can be expanded in powers of $\delta_n/\Omega_{R,n}$ as $\gamma = \frac{1}{T_2} + \gamma'\left(\delta_n/\Omega_{R,n}\right)$, where $\gamma'(\delta_n/\Omega_{R,n}) \to 0$ as $\delta_n/\Omega_{R,n} \to 0$. Introducing the inhomogeneous broadening, $S'_y(t_p)$ will be given by $S'_y\left(t_p\right) = e^{-t_p/T_2} \int g\left(\delta_n\right) a\, exp\left[-\gamma'\left(\delta_n/\Omega_{R,n}\right) t_p\right] d\delta_n$. The integral in the former expression can also be expanded as a power of $\gamma'(\delta_n/\Omega_{R,n})t_p$. In conclusion, $S'_y(t_p)$ can be given as $S'_y\left(t_p\right) \approx e^{-t_p/T_2} \sum_{k=0}^{\infty} a^{(k)} t_p^k$. In order to analyze our results, the summation in $S'_y(t_p)$ has been truncated up to $t_p^2$ terms. This approximation provides a good description of the experimental data. Besides, if the $exp(-t_p/T_2)$ factor is also expanded in powers of time, $S'_y(t_p)$ can be described by a polynomial expansion. Therefore, a second order

polynomial has been used to model the non oscillating contribution to $S_y(t_p)$, given by $S_y^{no}(t_p) = S'_y(t_p) + S_y^{st}$.

The oscillatory nutation signal $S_y(t_p)$ can described by Eq. (S2) provided that the length $t_p$ of the nutation pulse remains larger than $2\pi/\Omega_{R,n}$. On the other hand, as the pulses are non-ideal the effective nutation angle departs from the one expected for this equation for times $t_p < t_m$, $t_m$ being a threshold time. This effect can be taken into account by replacing $J_0(\Omega_{R,n}t_p)$ with $J_0(\Omega_{R,n}t_p - \Omega_{R,n}\, t_{p0})$ in Eq. (S2) where $t_{p0} \neq 0$ accounts for the effective shift in the nutation angle generated at short times. In the analysis, only data measured for $t_p > t_m$ can then be considered.

In conclusion, fits of the experimental data (see Fig. 3 and S8) are based on the function

$$S_y(t_p) = S_y^{no} + K_n e^{-t_p/\tau_{R,n}} J_0\left[\Omega_{R,n}\left(t_p - t_{p,0}\right)\right] \tag{S3}$$

with either (option I) $S_y^{no} = S_y^{st} + e^{-t_p/T_2}\left(a^{(0)} + a^{(1)}t_p + a^{(2)}t_p^2\right)$, or (option II) $S_y^{no} = b^{(0)} + b^{(1)}t_p + b^{(2)}t_p^2$. The choice of the function used to describe $S_y^{no}(t_p)$ does not significantly affect the values obtained for $\Omega_{R,n}$. By contrast, it introduces a small uncertainty in $\tau_{R,n}$. In spite of this, the dependence of $\tau_{R,n}$ on the Rabi frequency $\Omega_{R,n}$ remains qualitatively (and almost quantitatively) the same.

**Effect of spin-proton couplings on spin nutation signals** For some transitions and driving microwave powers, a second, virtually undamped, oscillatory signal is observed besides the “expected” damped oscillatory contribution (nutation signal). Detailed plots of $S_y(t_p)$ and its Fourier transform for transition 3 and HPA = 15 dB are shown in Fig. S9. These extra oscillations show up when the $^1$H nuclear Larmor frequency (18.3 MHz for $\mu_0 H_z$ = 0.43T) becomes close to the Rabi frequency of the relevant transition. This behavior has been

described before[S15] and it is associated with the hyperfine interaction of the electron spin with nearby protons. In order to take this effect into account, an additional term $S_H(t_p) = K_H \cos(\omega_H t_p + \varphi)$, has been added to Eq. (S3). In the fits, $\omega_H$ has been kept fixed and equal to the proton Larmor frequency.

**Calibration of the microwave magnetic field.** In order to get a precise determination of $h_1$ on the sample, a small crystal of the free radical BDPA has been attached to an $Y_{0.99}Gd_{0.01}W_{30}$ single-crystal and the spin nutation signals of both samples have been measured under identical experimental conditions, save for the tuning of their respective resonant magnetic fields. The crystals of both species were small enough (the long axis of the $Y_{0.99}Gd_{0.01}W_{30}$ single-crystal being about 1 mm and the other two about 0.3 mm) and were mounted with their larger axes pointing along the direction in which the microwave magnetic field of the cavity is nearly constant. Consequently it is safe to neglect effects derived from inhomogeneities in $h_1$. In the case of $Y_{0.99}Gd_{0.01}W_{30}$, transition 3 has been chosen by tuning $\mu_0 H_z$ to 430 mT. For this magnetic field, BDPA gives no contribution to the EPR signal. These measurements have been repeated two times in order to check the stability of the spectrometer. The results are shown in Fig. S10.

Due to the short coherence and relaxation times of BDPA, a relatively high $h_1$ was used (HPA = 10 dB) in order to ensure that the underdamped condition is fulfilled in this case. For $Y_{0.99}Gd_{0.01}W_{30}$, the nutation signal was fitted using Eq. (S3), option II. In the case of BDPA, we use $S_y(t_p) = S_y^{no}(t_p) + ce^{-\alpha_R t_p} \cos(\Omega_R t_p + \varphi)$, since this sample shows no significant inhomogeneous broadening. The Rabi frequencies obtained from the fits are $\Omega_{R,BDPA}/2\pi$ = (7.71±0.01) MHz for BDPA and $\Omega_{R,3}/2\pi$ = (30.31±0.05) MHz for $Y_{0.99}Gd_{0.01}W_{30}$. Using the gyromagnetic factor $g_{BDPA}$ = 2.003 of BDPA, we obtain $\mu_0 h_1$ =

(275 ± 5) μT. The ratio $\Omega_{R,3}/\Omega_{R,BDPA} \approx (g_{BDPA}\Omega_{R,3})/(g\Omega_R)$, with $g = 2$ for $Y_{0.99}Gd_{0.01}W_{30}$, provides a first estimation of the transition matrix element $a_3 = 3.93 \pm 0.08$.

In order to validate this procedure, the nutation signals of the outermost transitions of $Gd^{3+}$ impurities diluted in a single crystal of cubic $CaF_2$ have been used. This is a well characterized paramagnetic center for which the nutation frequencies of well isolated transitions can be calculated from the spin-Hamiltonian and from the measured relaxation times.[S16]

## Supplementary Figures

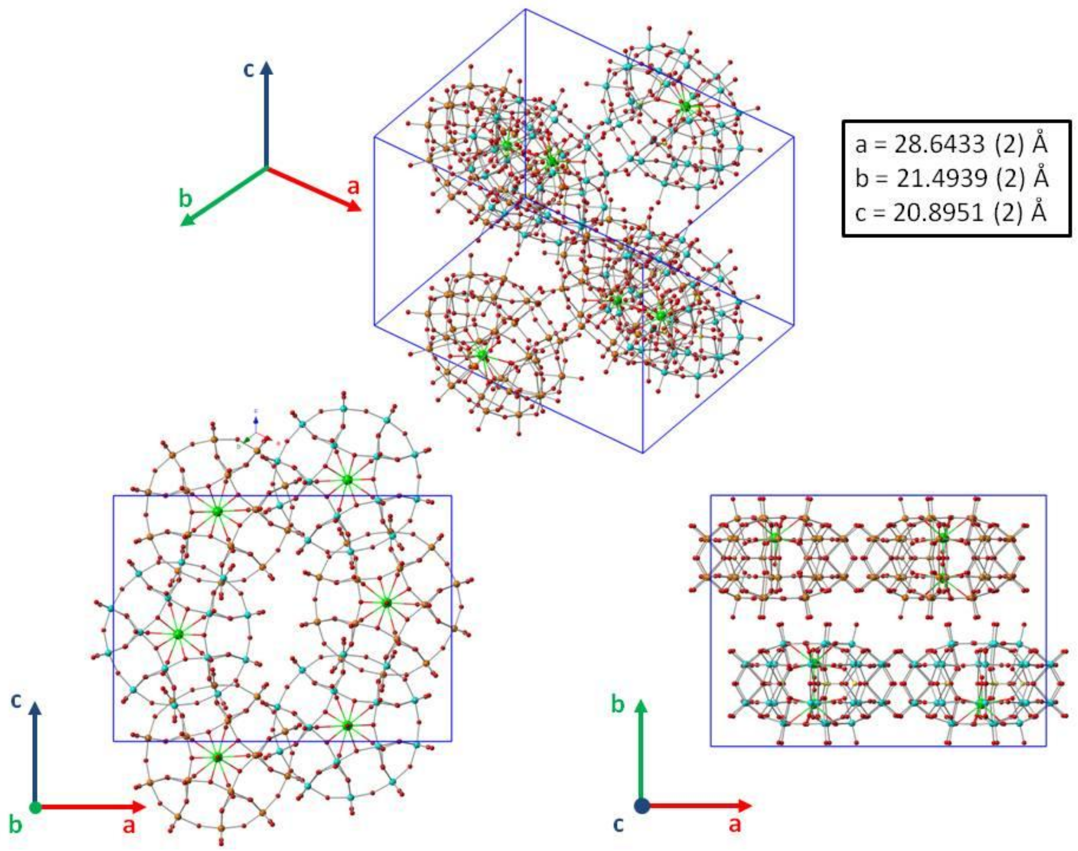


**Figure S1.** Crystal structure of $GdW_{30}$. The unit cell chosen contains 4 molecules.

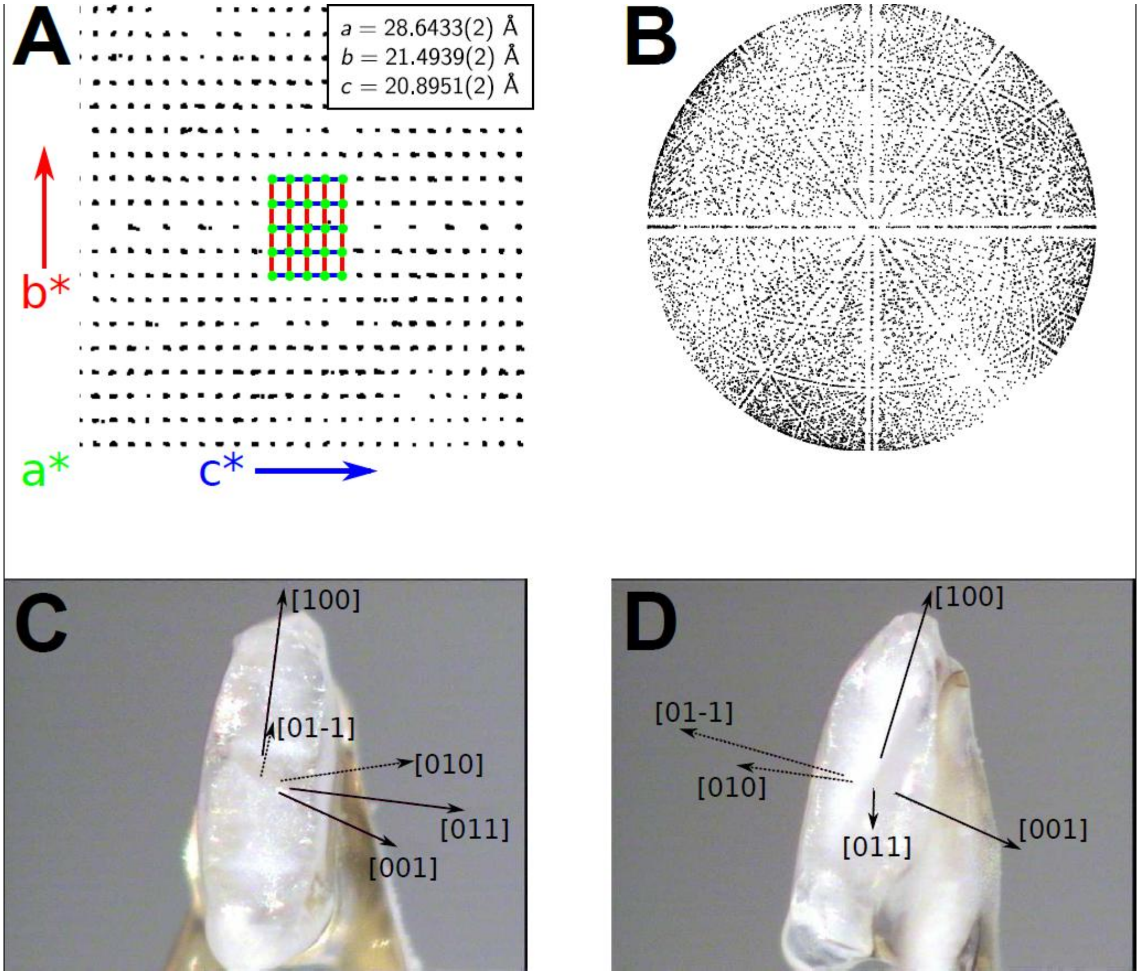


**Figure S2.** X-ray diffraction of magnetically diluted $Y_{0.99}Gd_{0.01}W_{30}$. Graph A shows the experimental reciprocal lattice and the lattice parameters. We find a good agreement with the orthorhombic structure described in Table S1. Graph B shows the experimental Ewald sphere. Graphs C and D show the orientation of several crystallographic axes with respect to the crystal facets, obtained from X-ray diffraction data.

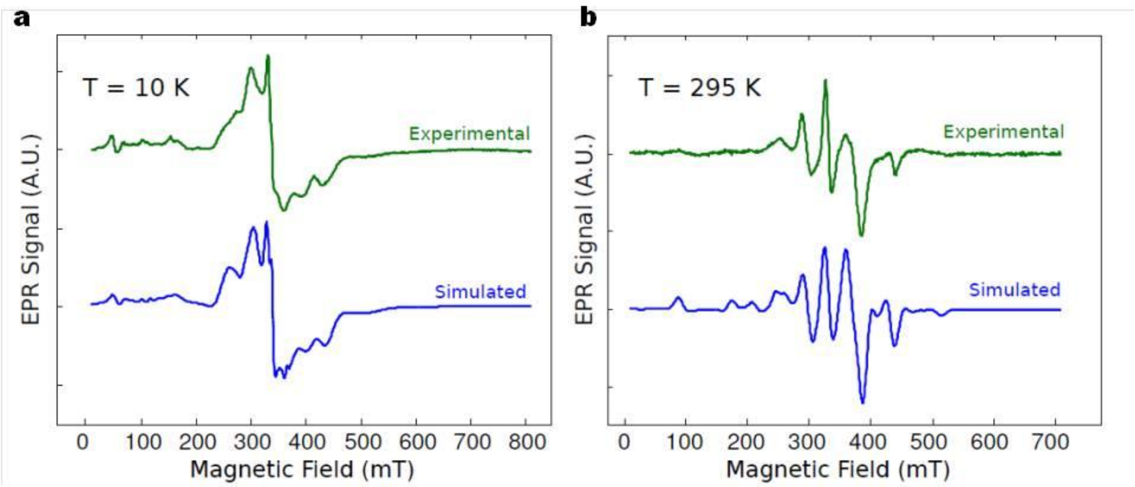


**Figure S3.** Powder X-band (9.475 GHz) cw-EPR spectra of $Y_{0.99}Gd_{0.01}W_{30}$. Experimental and simulated EPR spectra measured at $T$ = 10 K (**a**) and at $T$ = 295 K (**b**) on a powder sample ground from fresh crystals. The fits allow a determination of the magnetic anisotropy constants $D$ and $E$ of the spin Hamiltonian Eq. (1). The values found are $D$ = 1281 MHz and $E$ = 294 MHz at 10 K and $D$ = 1200 MHz and $E$ = 86 MHz at 295 K. Fitting the low-temperature data requires introducing sizeable strains in $D$ and $E$ parameters: $\Delta D$ = 330 MHz and $\Delta E$ = 224 MHz.

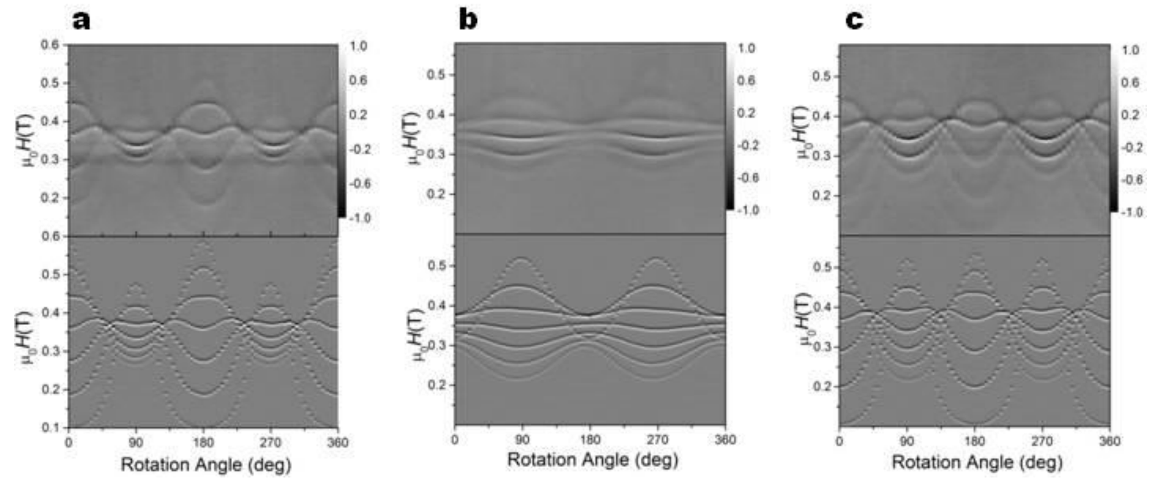


**Figure S4.** Angle-dependent electron paramagnetic resonance spectra. Experimental (top) and calculated (bottom) rotational X-band cw-EPR spectra measured at room temperature on a single crystal of $Y_{0.99}Gd_{0.01}W_{30}$. (**a**), (**b**) and (**c**) correspond to rotations along axes that are close to crystallographic axes [100], [011] and [01-1], respectively.

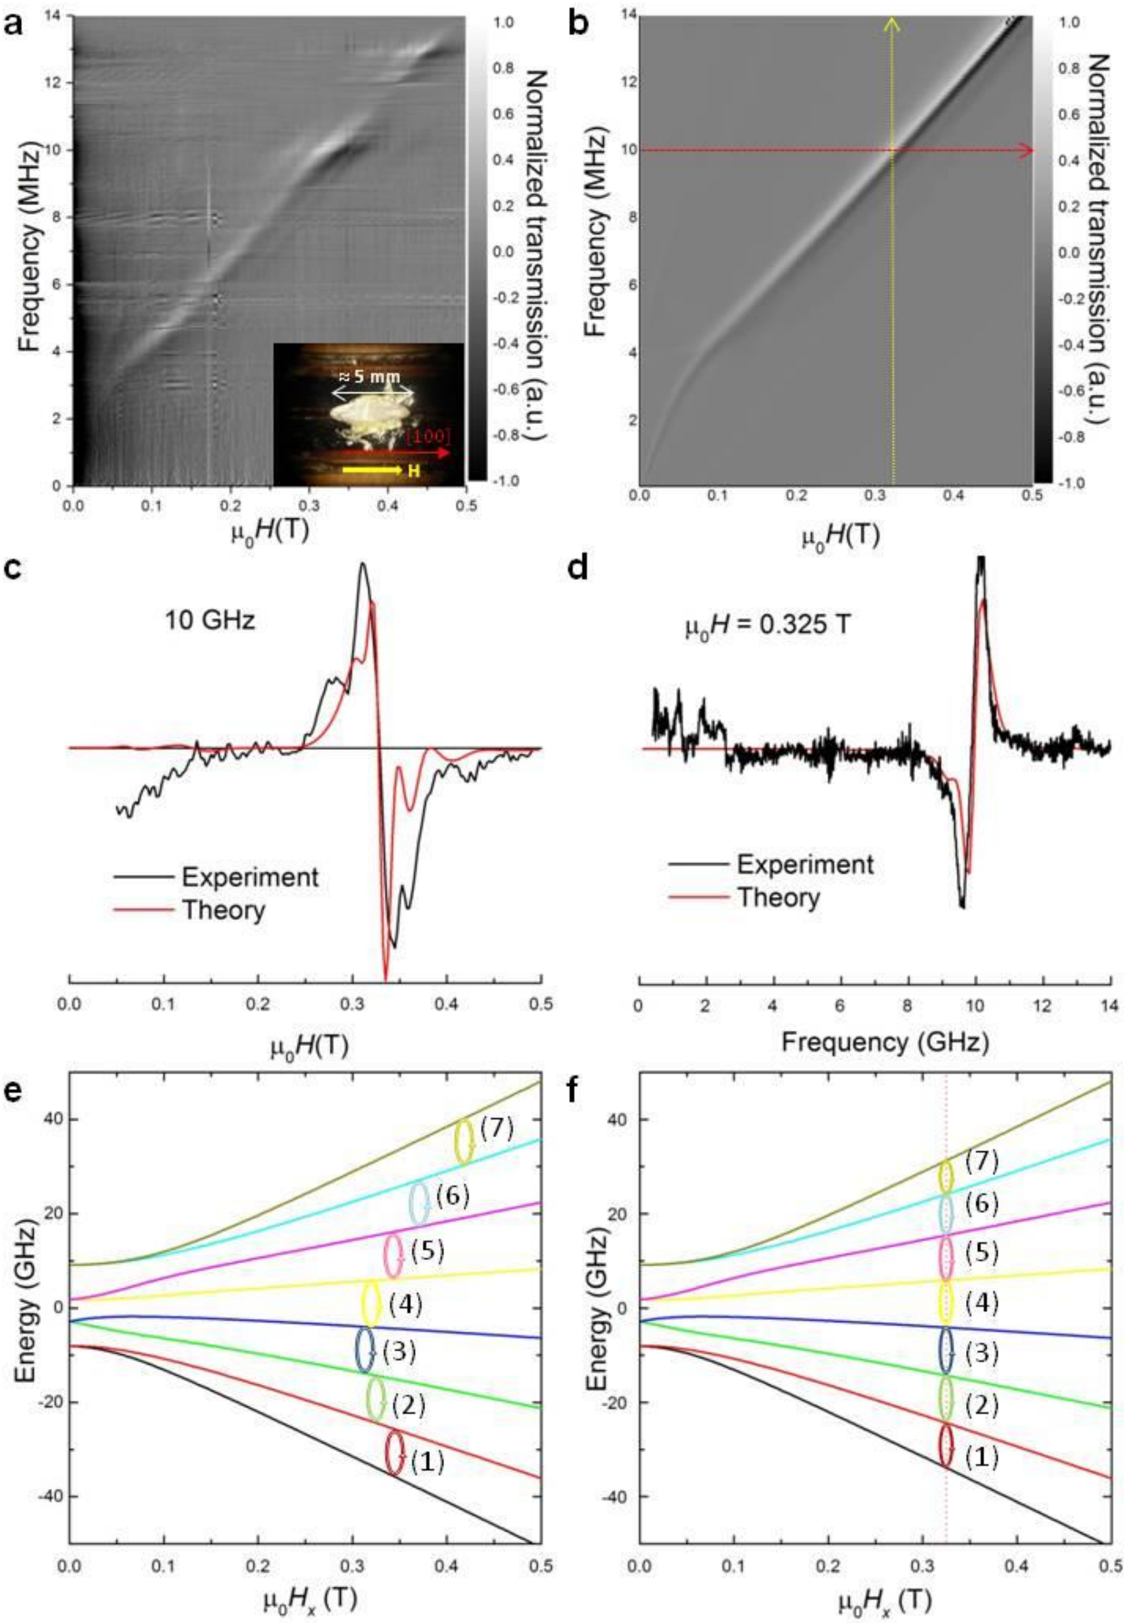
a
b
c
d
e
f
Frequency (MHz)
Normalized transmission (a.u.)
μ0H(T)
≈ 5 mm
[100]
H
10 GHz
μ0H = 0.325 T
Experiment
Theory
Frequency (GHz)
Energy (GHz)
μ0Hx (T)
(1)
(2)
(3)
(4)
(5)
(6)
(7)

**Figure S5.** Broad band magnetic spectroscopy with microwave transmission guides. (**a**) and (**b**) are, respectively, experimental and calculated 2D plots of the propagation of microwaves trough a coplanar superconducting transmission line (400 μm central line, 200 μm gap) that is coupled to a single crystal of $GdW_{30}$ oriented as shown in the inset. The magnetic field was applied along the **a** crystallographic axis, close to the medium magnetic axis **x**. The calculations have been made using the spin Hamiltonian (Eq. (1) in the main text) and the magnetic anisotropy parameters determined by powder EPR experiments (Fig. S7). (**c**) and (**d**) show traces obtained from these plots at, respectively, a fixed 10 GHz frequency as a function of magnetic field and at a fixed 0.325 T magnetic field as a function of frequency. These traces are indicated as arrows in (**b**). These experiments show that magnetic levels can be addressed by tuning either **H** or the microwave frequency ω, pointing to two possible protocols for operating between the logical states of a three qubit processor. These two protocols are shown in (**e**) (frequency fixed to 10 GHz) and (**f**) (magnetic field fixed to 0.325 T). The resonant magnetic fields in (**e**) are $\mu_0 H_x$ = 0.340 T, 0.324 T, 0.319 T, 0.323 T, 0.325 T, 0.343 T, and 0.423 T for transitions 1 to 7, respectively. The resonant frequencies in (**f**) are $\omega/2\pi$ = 9.545 GHz, 10.045 GHz, 10.177 GHz, 10.011 GHz, 9.547 GHz, 8.717 GHz, and 7.134 GHz for transitions 1 to 7, respectively.

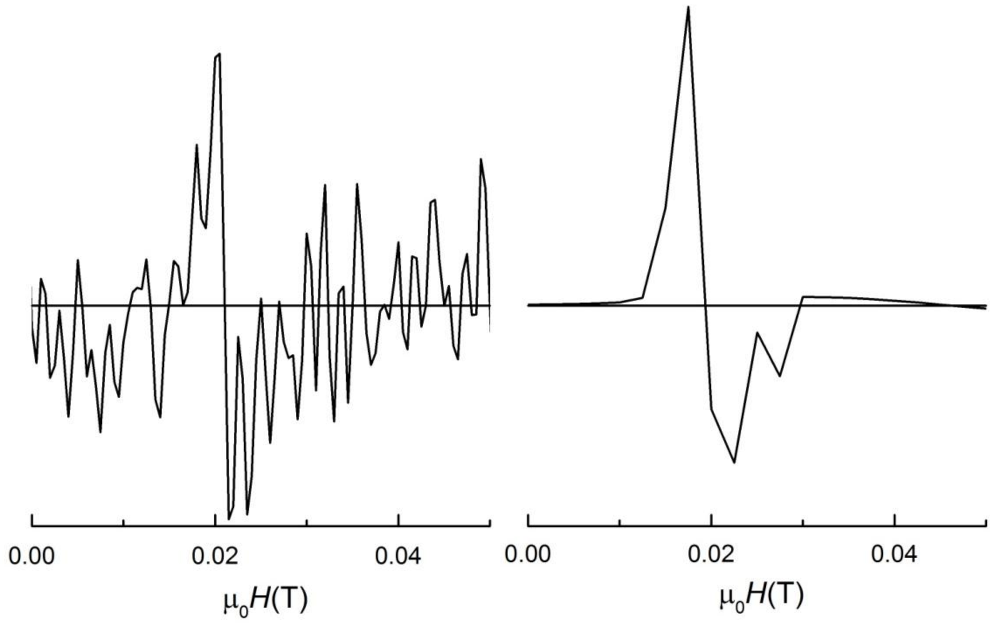


**Figure S6.** Coupling $GdW_{30}$ to a coplanar superconducting resonator. (**a**) and (**b**) show experimental and calculated resonance spectra obtained by coupling a single crystal of $K_{12}GdW_{30}$ to a 1.5 GHz coplanar superconducting resonator (central line 400 μm, gap 200 μm). The magnetic field was applied along the **a** crystallographic axis, close to the medium magnetic axis **x**. The calculations have been made using the spin Hamiltonian Eq. (1) and the magnetic anisotropy parameters determined by powder EPR experiments (Fig. S3).

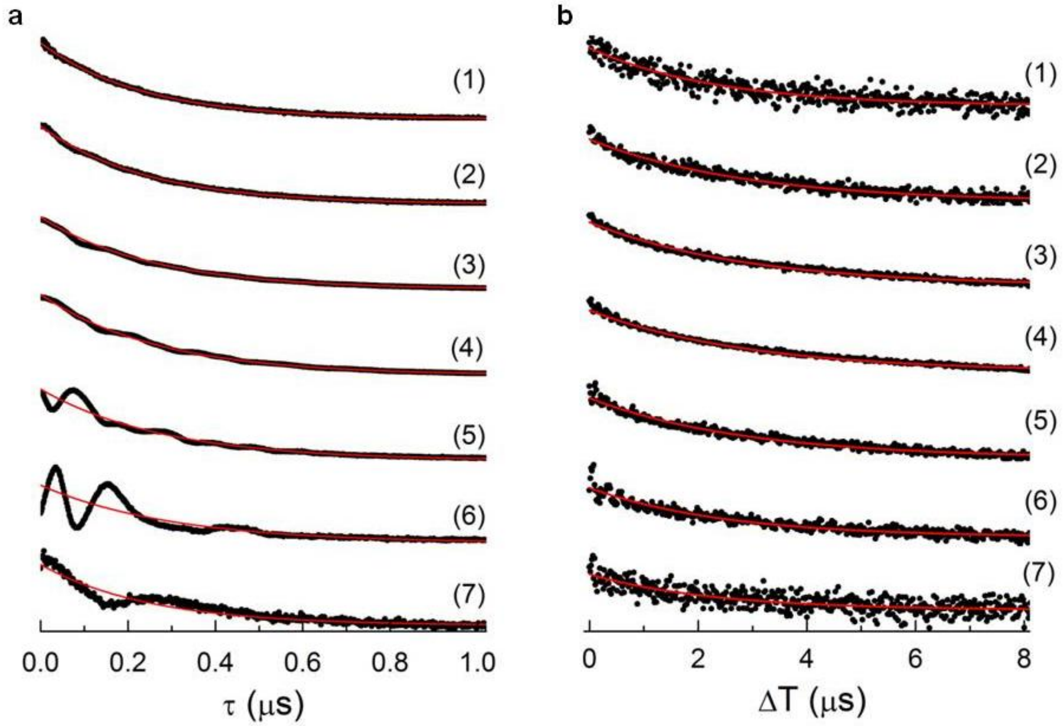


**Figure S7.** Experimental determination of spin coherence and spin-lattice relaxation times. (**a**) Decay of the echo amplitudes (dots) measured at $T$ = 6 K for transitions 1-7 after the application of a two-pulse Hahn-echo sequence. Each set of data is fitted with an exponential function (solid lines) from which the spin coherence times $T_2$ are extracted. (**b**) Decay of the echo intensities recorded at 6 K for each of the resonant transitions n = 1 to 7 after the application of a π/2-π/2-π/2 three-pulse sequence. The separation τ between the first two pulses was fixed to 100 ns whereas the separation T between the second and third pulses was varied between $T_0$ = 200 ns and 8 μs. Solid lines are least-squares fits to exponential functions from which the spin-lattice relaxation times $T_1$ are obtained.

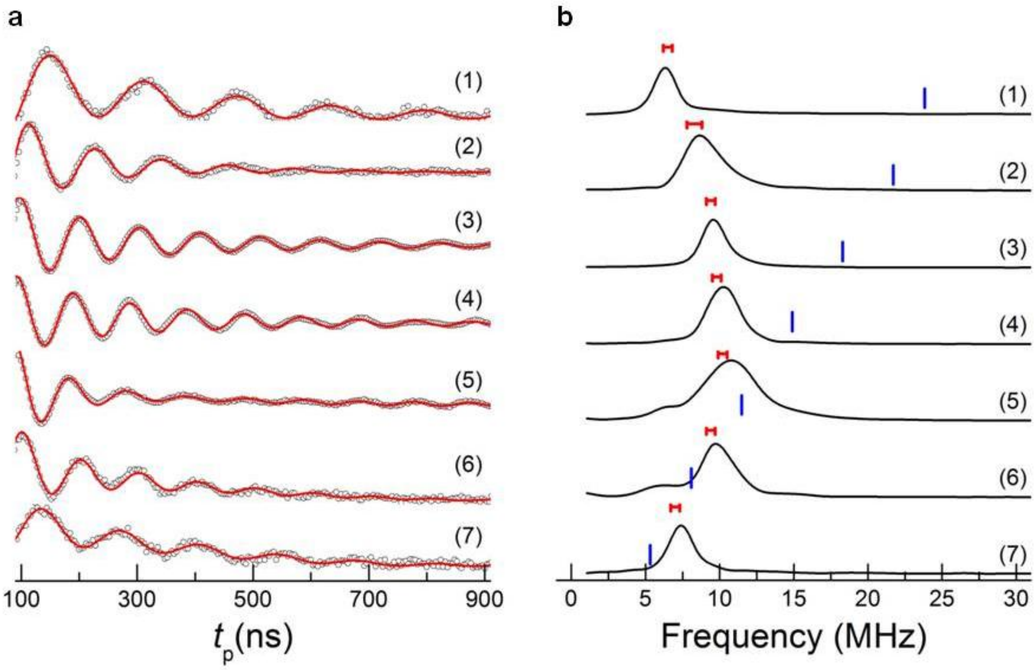


**Figure S8.** (**a**) Rabi oscillations for transitions 1 to 7 measured at $T$ = 6 K on a single crystal of $Y_{0.99}Gd_{0.01}W_{30}$ oriented as described in Figure 1a. The microwave power attenuation was HPA = 20 dB, corresponding to a microwave magnetic field amplitude $\mu_0 h_1$ = 92 ± 5 μT. The circles are experimental data and the solid lines are least-squares fits based on Eq. (3). (**b**) Digital Fourier transform (power spectrum) of the spin nutation signal in (**a**). The vertical sticks mark the Larmor frequency of the $^1$H nuclear spins at each magnetic field. The Rabi frequencies derived for each transition from the spin Hamiltonian (1) are given by solid dots.

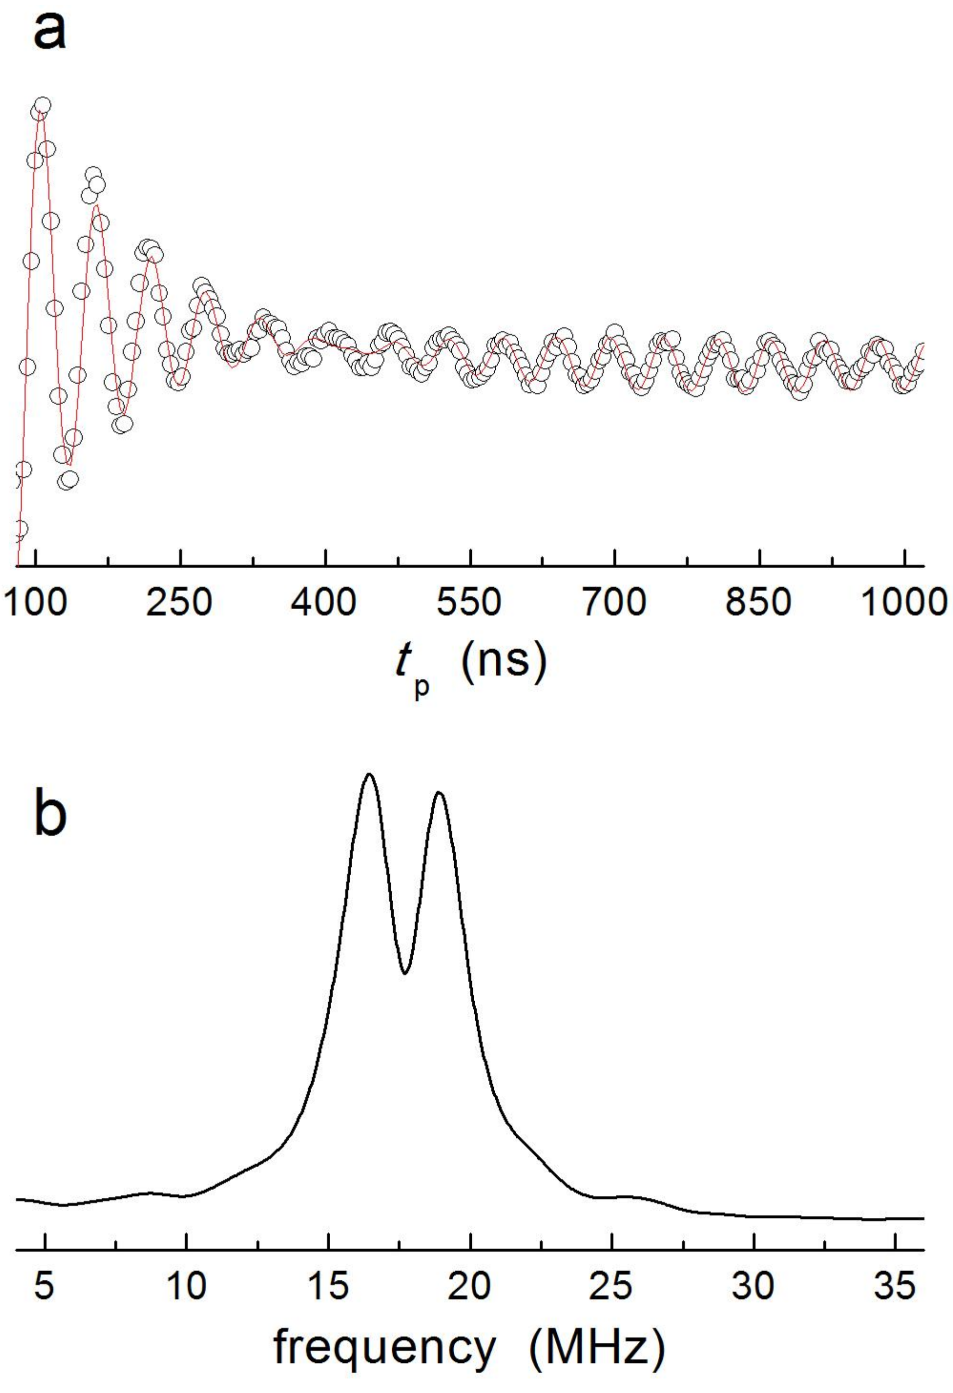


**Figure S9.** (**a**) Transient nutation of transition 3 (430 mT) measured at $T$ = 6 K on a single crystal of $Y_{0.99}Gd_{0.01}W_{30}$ with a microwave power attenuation HPA = 15 dB. The Rabi frequency $\Omega_{R,3}/2\pi$ = 17.13 MHz of the damped oscillations is close to the $^1$H nuclear Larmor frequency $\omega_H/2\pi$ = 18.31 MHz, which corresponds to the frequency of the virtually

undamped oscillations observed at long times. (**b**) Fourier transform (power spectrum) of the nutation signal shown in (**a**).

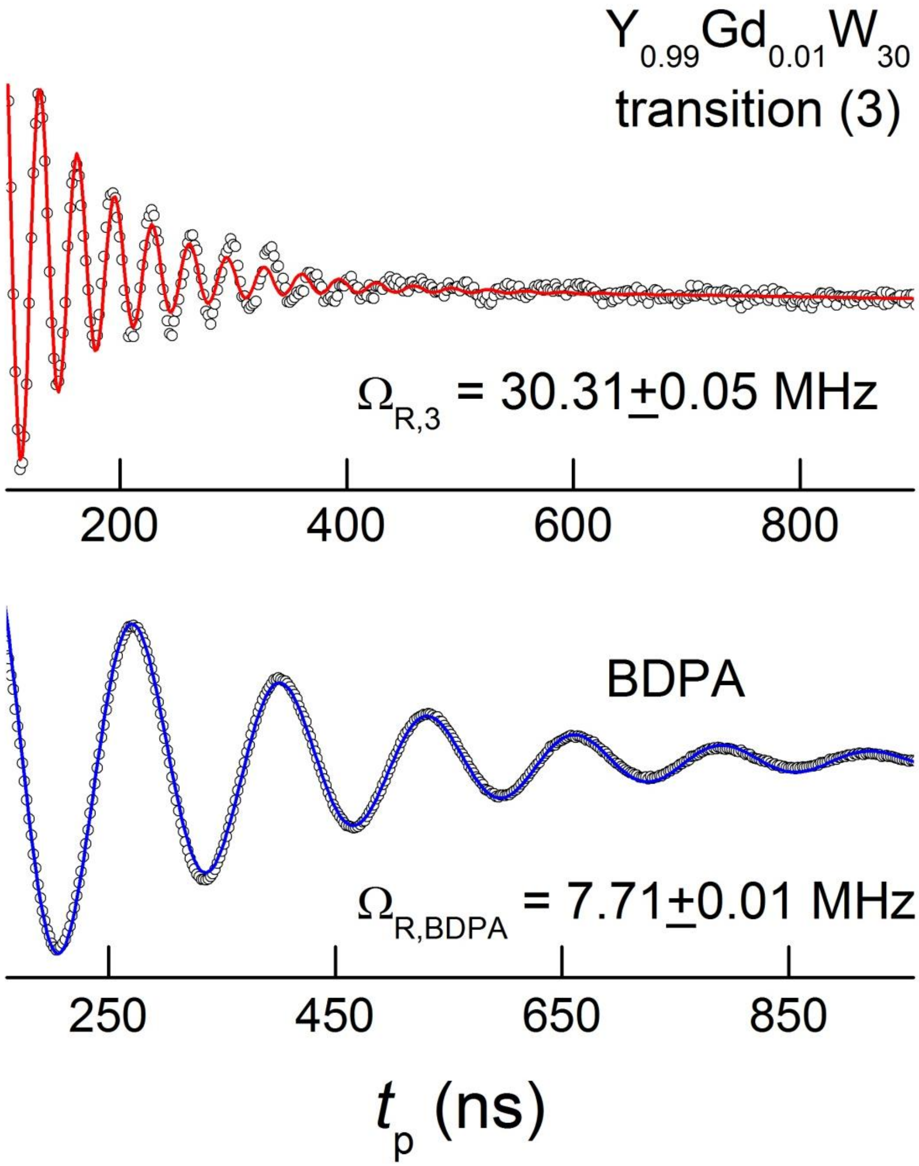


**Figure S10.** Calibration of the microwave magnetic field. (**a**) Spin nutation signal of transition 3 measured at $T$ = 6 K on an $Y_{0.99}Gd_{0.01}W_{30}$ single crystal oriented as shown in Fig. 1a. (**b**) Spin nutation signal of a BDPA radical sample attached to the former crystal, measured at the same temperature by detecting the free induction decay signal. Circles are experimental data whereas solid lines are least squares fits based on Eq. (S3), option II, for $Y_{0.99}Gd_{0.01}W_{30}$ and on $S_y(t_\mathrm{p}) = S_y^\mathrm{no}(t_\mathrm{p}) + ce^{-t/\tau_\mathrm{R}} cos\left(\Omega_\mathrm{R} t_\mathrm{p} + \varphi\right)$ for BDPA.

## Supplementary Tables

**Table S1**. Crystallographic data for $GdW_{30}$ and $YW_{30}$.

| Compound | $GdW_{30}$ | $YW_{30}$ |
|---|---|---|
| Empirical formula | $GdH_{57}K_{12}O_{138.5}P_5W_{30}$ | $YH_{60}K_{12}O_{140}P_5W_{30}$ |
| Formula weight | 8570.25 | 8528.94 |
| Space group | P*nma* | P*nma* |
| $a$ (Å) | 28.6500(3) | 28.7746(4) |
| $b$ (Å) | 21.4914(2) | 21.4999(2) |
| $c$ (Å) | 20.89261(18) | 20.88851(17) |
| $\alpha$ (deg.) | 90 | 90 |
| $\beta$ (deg.) | 90 | 90 |
| $\gamma$ (deg.) | 90 | 90 |
| $V$ (Å$^3$) | 12864.2(2) | 12922.7(2) |
| $Z$ | 4 | 4 |
| $T$ (K) | 120.00(10) | 120.00(10) |
| $\lambda$ (Å) | 0.71073 | 0.71073 |
| $\rho_{calc}$ (g cm$^{-3}$) | 4.425 | 4.384 |
| $\mu$ (mm$^{-1}$) | 27.782 | 27.596 |
| $R[F_o^2 > 2\sigma(F_o^2)]^a$ | 0.0567 | 0.0580 |
| $R_w[F_o^2 > 2\sigma(F_o^2)]^b$ | $0.1154^c$ | $0.1239^d$ |

$^a$ $R = \Sigma(||F_o| - |F_c||)/\Sigma|F_o|$. $^b$ $R_w = \{\Sigma[w(F_o^2 - F_c^2)^2]/\Sigma[w(F_o^2)^2]\}^{1/2}$. $w = 1/[\sigma^2(F_o^2) + (AP)^2 + BP]$, where $P = (F_o^2 + 2F_c^2)/3$. $^c$ $A = 0.0203$, $B = 905.3145$. $^d$ $A = 0.0410$, and $B = 585.1000$.

**Table S2.** Unit cell parameters of $Y_{1-x}Gd_xW30$ ($x$ = 0.01 and 0.05), measured at 120 K.

| Compound | $Y_{0.99}Gd_{0.01}W_{30}$ | $Y_{0.95}Gd_{0.05}W_{30}$ |
|---|---|---|
| $a$ (Å) | 28.796(4) | 28.780(4) |
| $b$ (Å) | 21.507(4) | 21.483(3) |
| $c$ (Å) | 20.887(4) | 20.898(3) |
| $\alpha$ (deg.) | 90 | 90 |
| $\beta$ (deg.) | 90 | 90 |
| $\gamma$ (deg.) | 90 | 90 |
| $V$ (Å$^3$) | 12936(4) | 12921(3) |

## References


S1 Creaser, I.; Heckel, M.; Neitz, R.; Pope, M. *Inorg. Chem.* **1993**, 32, 1573−1578.

S2 Sheldrick, G. M. SHELXTL Version 2014/7. http://shelx.uni-ac.gwdg.de/SHELX/index.php.

S3 Schweiger A.; Jeschke G. *Principles of Pulse Electron Paramagnetic Resonance*; Oxford University Press: New York, 2001; Chapter 14.

S4 Baibekov, E. I. *Appl. Magn. Reson*. **2014**, 45, 1289-1297.

S5 Baibekov, E. I. *JETP letters* **2011**, 93, 292-297.

S6 Torrey H. C. *Phys. Rev*. **1949**, 76, 1059-1068.

S7 Boscarino, R.; Gelardi, F. M.; Mantegna, R. N. *Phys. Lett. A* **1987**, 124, 373-376.

S8 Boscarino, R.; Gelardi, F. M.; Korb, J. P. *Phys. Rev. B* **1993**, 48, 7077-7085.

S9 Shakhmuratov, R. N.; Gelardi, F. M.; Cannas, M. *Phys. Rev. Lett*. **1997**, 79, 2963-2966.

S10 Asadullina, N. Ya.; Asadullin, .T. Ya.; Asadullin, Ya. Ya. *J. Phys: Condens. Matter* **2001**, 13, 3475-3489.

S11 Agnello, S.; Boscarino, R.; Cannas, M.; Gelardi, F. M.; Shakhmuratov, R. N. *Phys. Rev. A* **1999**, 59, 4087-4090.

S12 Baibekov, E. I.; Gafurov, M. R.; Zverev, D. G.; Kurkin, I. N.; Malkin B. Z.; Barbara, B. *Phys. Rev. B* **2014**, 90, 174402 (1-9).

S13 Baibekov, E. I. *J. Supercond. Nov. Magn*. **2013**, 26, 1595-1597.

S14 De Raedt, H.; Barbara, B.; Miyashita, S.; Michielsen, K.; Bertaina, S.; and Gambarelli, S. *Phys. Rev. B* **2012**, 85, 014408 (1-17).

S15 Baldoví, J. J.; Cardona-Serra, S.; Clemente-Juan, J. M.; Coronado, E.; Gaita-Ariño, A.; and Prima-García, H. *Chem. Commun.* **2013**, 49, 8922-8924.

S16 Arauzo A. B., Alcalá R., Alonso P. J. *Appl. Mag. Reson*. **12**, 375-387 (1997).
